# Supplementary material for: Modelling Dynamic Interactions between Relevance Dimensions
Source: arXiv:1907.10943 source file (2019-07-25)
Supplement: Supplementary file 1 [file appendix.tex]

\appendix
\section{Appendix}
Consider a state vector in two different basis of a two dimensional Hilbert space, $\ket{\psi} = a\ket{A}+b\ket{B} = c\ket{C}+d\ket{D}$
We want to represent the vectors of one basis in terms of the other. To do that, consider the vector orthogonal to $\ket{\psi}$, which is $\ket{\widetilde{\psi}} = b\ket{A}-a\ket{B} = d\ket{C}-c\ket{D}$. Using the above representations, we get 
\vspace{-2mm}
\begin{equation}\label{c,d}
\ket {C} = c\ket{\psi} + d\ket{\widetilde{\psi}} and 
\ket {D} = d\ket{\psi} - c\ket{\widetilde{\psi}}
\end{equation}
\vspace{-2mm}
Substituting $\ket{\psi} = a\ket{A}+b\ket{B}$ and $\ket{\widetilde{\psi}} = b\ket{A}-a\ket{B}$ in \ref{c,d}, we get:
\begin{align}
\ket {C} &= (ac+bd)\ket{A} + (bc-ad)\ket{B} \nonumber \\
\ket {D} &= (ad-bc)\ket{A} + (ac+bd)\ket{B}
\end{align}
